# Supplementary material for: Bubble growth in a confined heated polymer: the example of safety glass
Source: arXiv:2412.04617 source file (2026-01-21)
Supplement: Supplementary file 1 [file Why_does_safety_glass_bubble_supp_mat.pdf]

## Supplementary Material: Why does safety glass Bubble?

Carlos Arauz-Moreno<sup>1,2</sup>, Keyvan Pirorid<sup>2</sup>, & Elise Lorenceau<sup>1</sup>

### Rheology of PVB polymers

We surveyed the rheological behavior of RB41, QS41, and DG41 in the frequency space using oscillatory shear rheometry ( $\omega=0.1-10$  rad/s), under small deformation ( $Y=0.01\%$ ), and between 20-140°C. From the time-temperature master curves, we derived two characteristic times  $t_e, t_d$ . The former denotes the Rouse relaxation, and thus, the transition from the glassy to the rubbery state. The latter is the characteristic time of reptation of the polymer chains and signals accordingly the rubbery-to-viscous transition. These times scale with temperature and are thus used to create a time-temperature diagram for the polymers under small strain. See Arauz-Moreno, Piroird, & Lorenceau (2022) for information on the experimental protocol, sample preparation, and relevant equations used to create the diagrams.

Concerning the Rouse transition, for QS41 (tri-layer) we found two relaxation times (25°C)  $t_{e,A} \approx 19.3$  s and  $t_{e,B} \approx 0.12$  s, which signal that two layers are identical in relaxation, while the third one is not. The longest Rouse time in this case was fairly identical to one for RB41 ( $t_e \approx 20$  s) which suggests that the layers in question may be of identical composition. The Rouse time for DG41 was in the order of  $\approx 3.45 \times 10^5$  s, which reflects the reduced amount of plasticizer in this blend, and hence, its stiffer nature. In terms of the reptation times, the blends exhibited widely different values of  $t_d = 10^{12}$  s (DG41),  $10^9$  s (RB41), and  $10^8$  s (QS41).

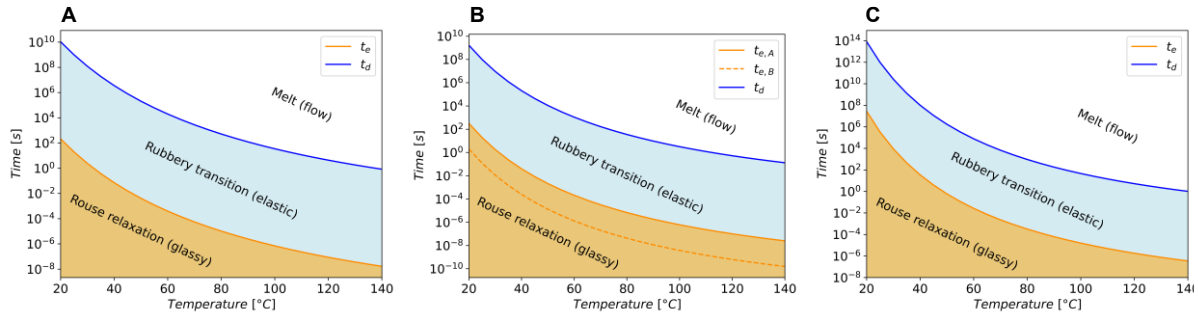

Figure 1: Time-temperature state diagram for PVB polymers. **A** RB41, **B** QS41, **C** DG41. The transition is delineated by  $t_e$  and  $t_d$ , the Rouse and reptation time of the polymer chains respectively.

The generalized time-temperature Maxwell model for RB41 (and RB11 for they have the same chemistry), includes 10 spring elements, with an equal number of relaxation times. The constants are:

Table 1: Maxwell model constants at  $T_r=25^\circ\text{C}$  (Arauz-Moreno et al, 2021)

| $G_i[\text{Pa}]$ | $\lambda_i[\text{s}]$ | $G_i[\text{Pa}]$ | $\lambda_i[\text{s}]$ |
|------------------|-----------------------|------------------|-----------------------|
| 3.40E+06         | 3.34E−01              | 8.42E+04         | 1.52E+08              |
| 8.09E+05         | 6.56E+00              | 3.65E+04         | 1.23E+09              |
| 1.92E+05         | 4.59E+02              | 1.14E+04         | 8.90E+09              |
| 1.13E+05         | 2.56E+05              | 2.38E+03         | 6.69E+10              |
| 1.08E+05         | 1.02E+07              | 4.23E+02         | 4.84E+11              |

## Water content post lamination

The amount of water dissolved in the PVB bulk can be measured along the lamination process via near infrared (NIR) spectroscopy. It simply suffices to take a reference spectrum of glass without PVB (preferably of equivalent thickness as the sample to be measured), and then scan either a pre-press or a finished sample of laminated safety glass. The qualitative amount of water is  $r_{abs} = p_{H_2O}/p_{PVB}$ , where  $p$  is the transmission peak for water (1873-1925 nm) and PVB (1609-1710 nm) respectively (figure S2A). See Arauz-Moreno, Piroird, & Lorenceau (2023) for further details.

As shown in figure S2B, post autoclaving, the amount of water from the pre-press to the finished sample is roughly the same, except around the edges. In this respect, water is lost because of mass diffusion. The affected length is only a couple of millimeters, however.

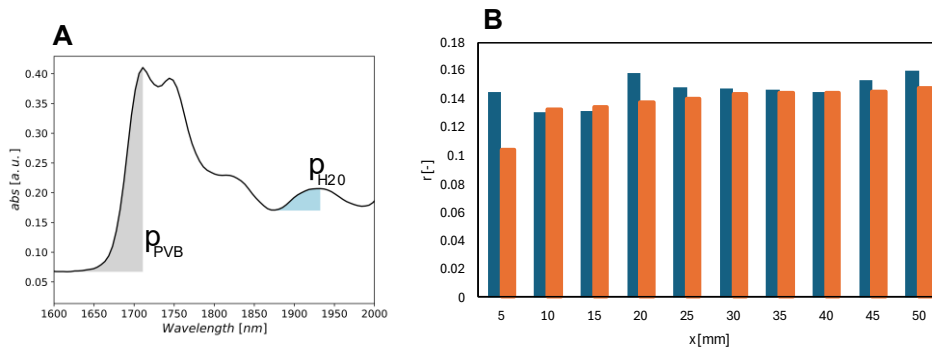

Figure 2: **A** Typical NIR spectrum in a glass sample with PVB. **B** NIR spectra of a sample, before (blue bars) and after autoclaving (orange bars).  $x=0$  is the edge of the glass sample. Water is lost (only) around the edges because of mass diffusion).

## Experimental set-up

We developed a set of transparent, cylindrical autoclave cells to visualize glass samples under complex schedules of temperature and pressure. The primary cell—here autoclave A (figure S3A)—was made from aluminum and included a set of viewing windows, as well as dedicated ports for supplying pressure (Fluigent pressure generator) and heat using silicon oil as the thermal fluid (Unistat thermobath). This cell is capable of providing active cooling. A camera was placed overhead to record images using a high magnification objective (105 mm) and illumination was provided from below using an LED light source with a mirror at 45°. The temperature was controlled via a set of PT100 sensors placed directly on the sample at two locations (figure S3B). The edge temperature T1 was used as part of the control loop of the system to regulate the temperature of the silicon oil. The T2 temperature was deemed representative of the target imaging area where we took our bubble measurements. The secondary cell, autoclave B (not shown) was made from stainless steel, heat was provided via a set of heating ropes (no cooling), and the magnification was smaller (75 mm objective). Only the equivalent of temperature T1 was measured (15 mm from the edge). Hence, a calibration was made to match this temperature to the T2 temperature from autoclave A. Finally, we tracked bubbles in three separate regions of interest (ROIs) inside small target imaging area of the sample. The analysis was then performed using ImageJ and python.

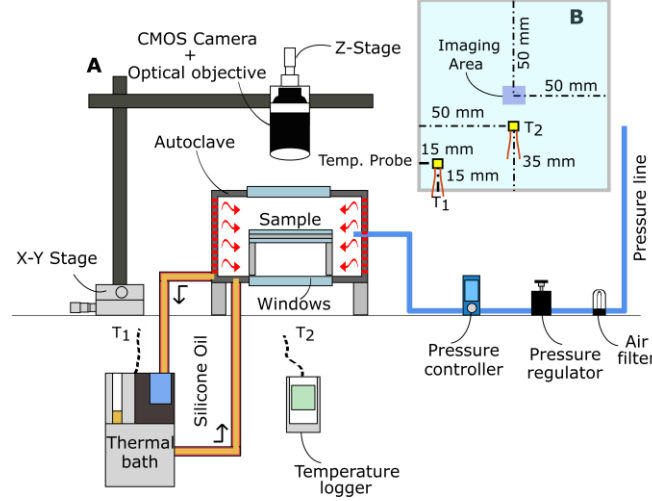

Figure 3: **A** Transparent autoclave set-up. **B** Glass sample schematics detailing the relevant temperature measurements and the target area whence the bubble images are taken.

### Mass Transport in PVB: air and water

Table 2 presents the physical constants for air and water used in the bake test simulations. Air properties can be found in Arauz-Moreno, Piroird, & Lorenceau (2024). The corresponding ones for water are found in Arauz-Moreno, Piroird, & Lorenceau (2022). Water transport in PVB depends strongly on temperature and moisture. In particular, water has a variable activation energy of diffusion  $E_d(T)$ , which we simplified here by taking an average value  $E_{d,avg}$  from the range of 20-140°C. The diffusion coefficient is likewise moisture dependent. Hence, the Arrhenius expression was taken as

$$\ln\left(\frac{D}{D_{ref}}\right) = -\frac{E_{d,avg}}{R_u}\left(\frac{1}{T} - \frac{1}{T_r}\right) - \gamma(a - a_r)$$

where  $\gamma = -1.4$  and  $a_r = 0.0907$ .

Table 2: Mass transport constants

|              | Air                    | Water vapour          |
|--------------|------------------------|-----------------------|
| $T_{ref}$    | 20°C                   | 25°C                  |
| $H_{ref}$    | $5.92 \times 10^{-7}$  | $5.96 \times 10^{-3}$ |
| $\Delta H_s$ | 5.0                    | -42                   |
| $D_{ref}^*$  | $4.38 \times 10^{-11}$ | $1 \times 10^{-11}$   |
| $E_d$        | 20.6                   | 47                    |

\* Diffusion coefficient for water at  $a_{ref} = 0.0907$ .

## Nucleation in finished glass

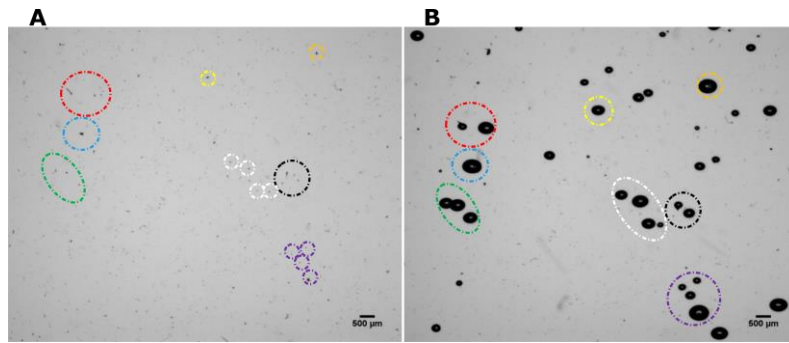

Figure 4: Autoclave images of faulty LSG samples. **A** Before bake testing (16hrs, 100°C). **B** Post bake testing. The circle areas help identify the location of gas nuclei.
